# Supplementary material for: A Vehicle System for Navigating Among Vulnerable Road Users Including Remote Operation
Source: arXiv:2505.04982 source file (2025-05-08)
Supplement: Supplementary file 1 [file appendix.tex]

\section{Appendix}\label{sec:appendix}

\hl{Dariu@all: this section will be removed completely and I will add a sentence in the paper reminding the reviewers of a combined video we have as supplemental material.}

\DMG{Here we list a set of supporting materials that help assess various system components or earlier system versions:}
\todo{Dariu@all: Please add them to Surfdrive under IV-All / Publications / 2024 / RSS'2024. and provide a short description for each here (say 3 lines max).}

\begin{itemize}

\item The video \texttt{Test\_localization\_2023-12-19.mp4} demonstrates the localization stack. The system can already accurately determine the vehicle's position w.r.t.~the 3D map.

\item \barys{The video \texttt{Prius\_HoekvanHolland.mp4} demonstrates automated maneuvers such as Double Lane Change in poor weather conditions. The controller is able to accurately follow the predefined trajectory on the slippery surface.}

\item \oscar{The video \texttt{motion-planning.mp4} demonstrates the motion planner. It shows how the motion planner, consisting of a single probabilistic local planner, navigates among four virtual pedestrian with uncertain dynamics.}
\end{itemize}
